# Supplementary material for: Penalized regression calibration: a method for the prediction of survival outcomes using complex longitudinal and high-dimensional data
Source: arXiv:2101.04426 source file (2021-09-29)
Supplement: Supplementary file 1 [file supplementary_material_prc_v3.pdf]

Supplementary material of the article  
“Penalized regression calibration: a method for the prediction of survival  
outcomes using complex longitudinal and high-dimensional data”

Mirko Signorelli<sup>1</sup>, Pietro Spitali<sup>2</sup>, Cristina Al-Khalili Szigyarto<sup>3</sup>, The MARK-MD Consortium,  
and Roula Tsonaka<sup>1</sup>

<sup>1</sup>*Department of Biomedical Data Sciences, Leiden University Medical Center (NL)*

<sup>2</sup>*Department of Human Genetics, Leiden University Medical Center (NL)*

<sup>3</sup>*Department of Protein Science, KTH-Royal Institute of Technology (SW)*

# 1 Supplementary Figures

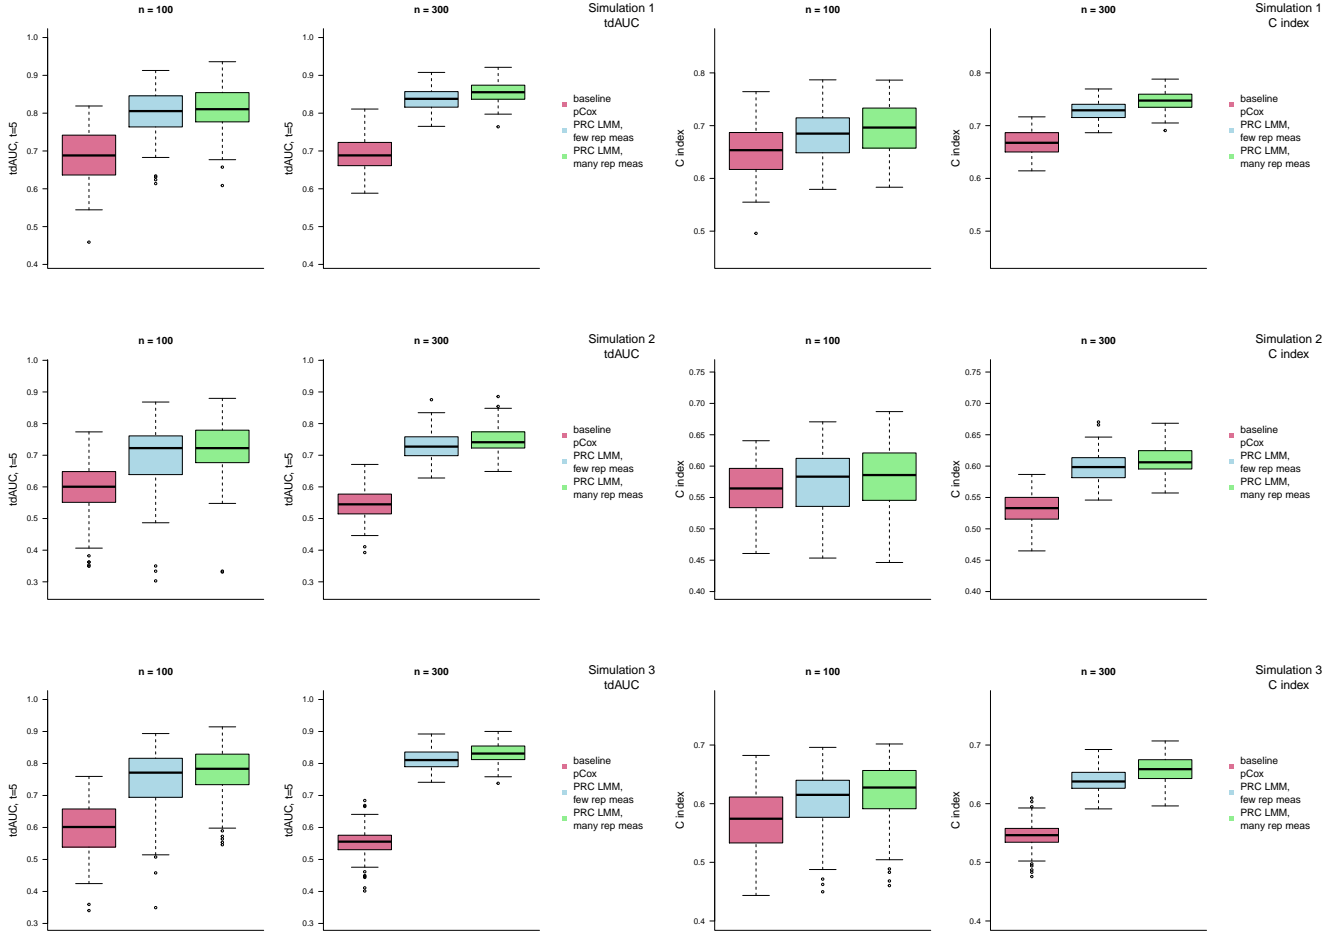

Figure 1: Results of simulations 1, 2 and 3 using the elasticnet penalty. The boxplots compare the distribution over 100 random replications of the optimism-corrected tdAUC (left) and C index (right) of the PRC LMM model when few (lightblue) or many (lightgreen) repeated measurements are available to that of a penalized Cox model where only baseline measurements are used (violet red).

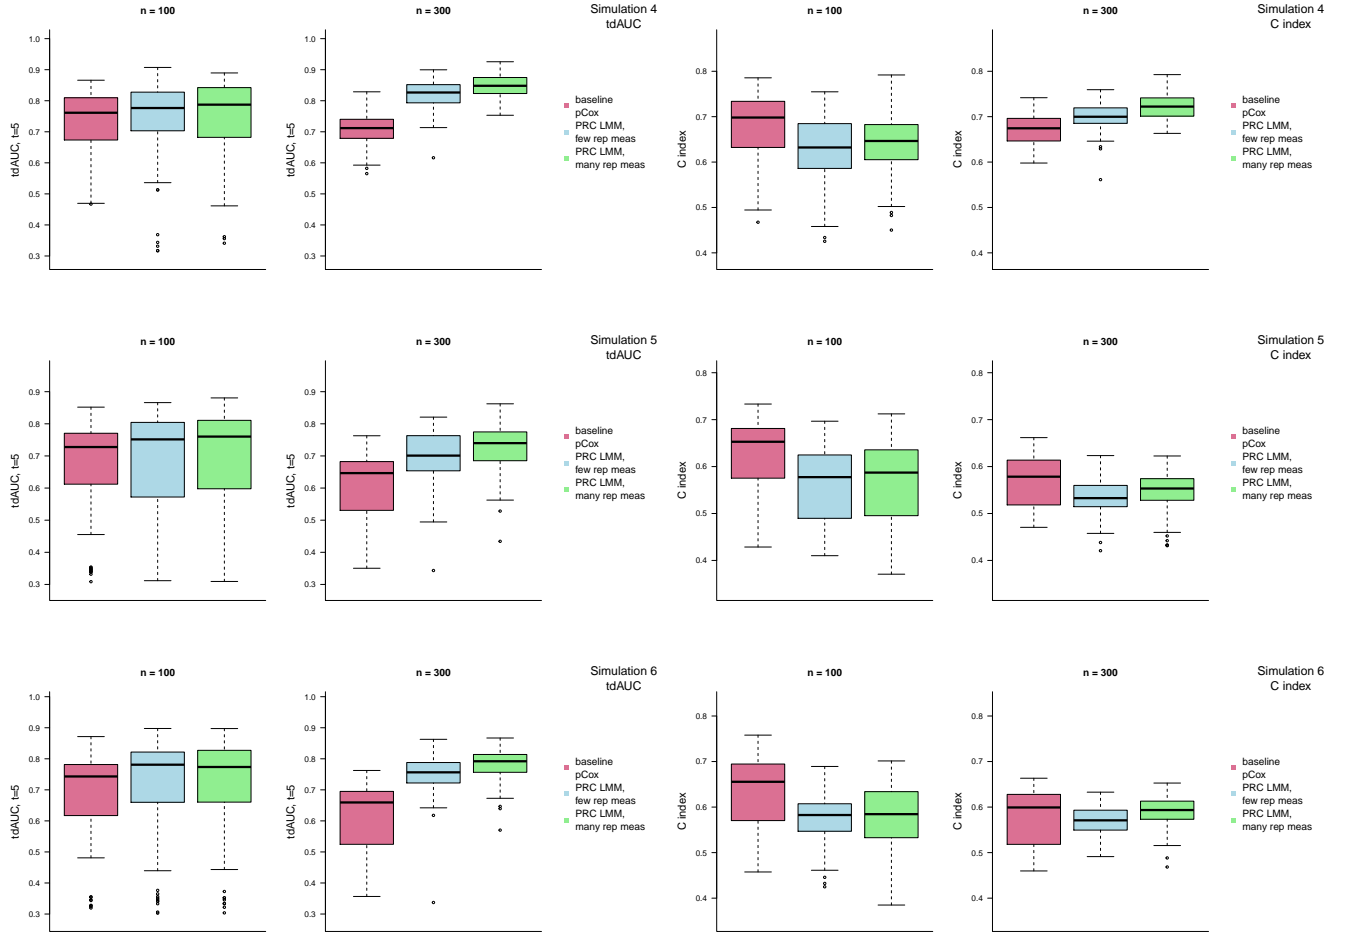

Figure 2: Results of simulations 4, 5 and 6 using the elasticnet penalty. The boxplots compare the distribution over 100 random replications of the optimism-corrected  $tdAUC$  (left) and C index (right) of the PRC LMM model when few (lightblue) or many (lightgreen) repeated measurements are available to that of a penalized Cox model where only baseline measurements are used (violet red).

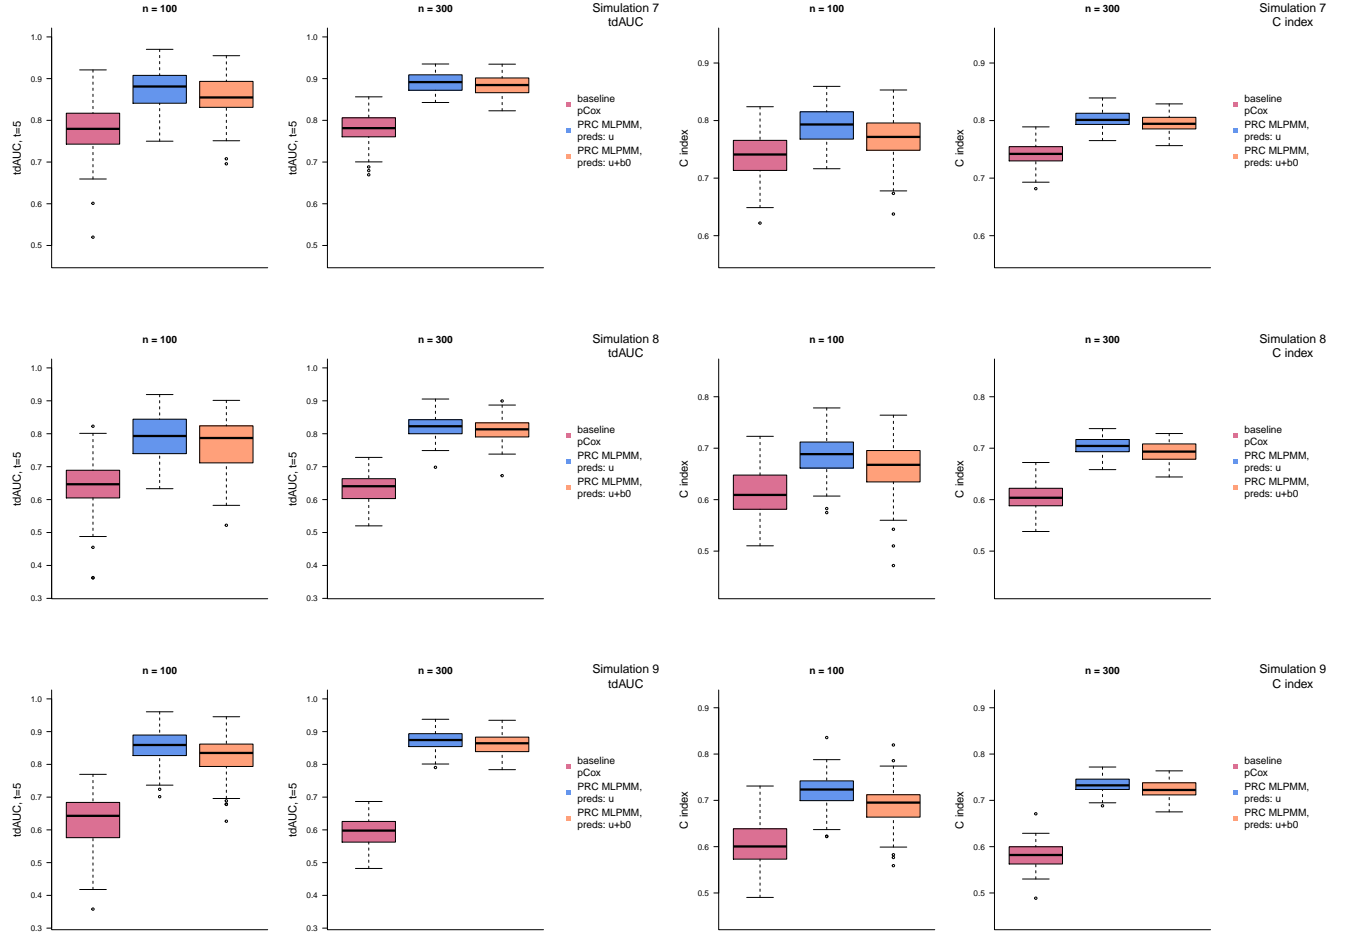

Figure 3: Results of simulations 7, 8 and 9 using the elasticnet penalty. The boxplots compare the distribution over 100 random replications of the optimism-corrected  $tdAUC$  (left) and C index (right) of the baseline pCox (violet red), PRC-MLPMM(U) (blue) and PRC-MLPMM(U+B) (orange) models.

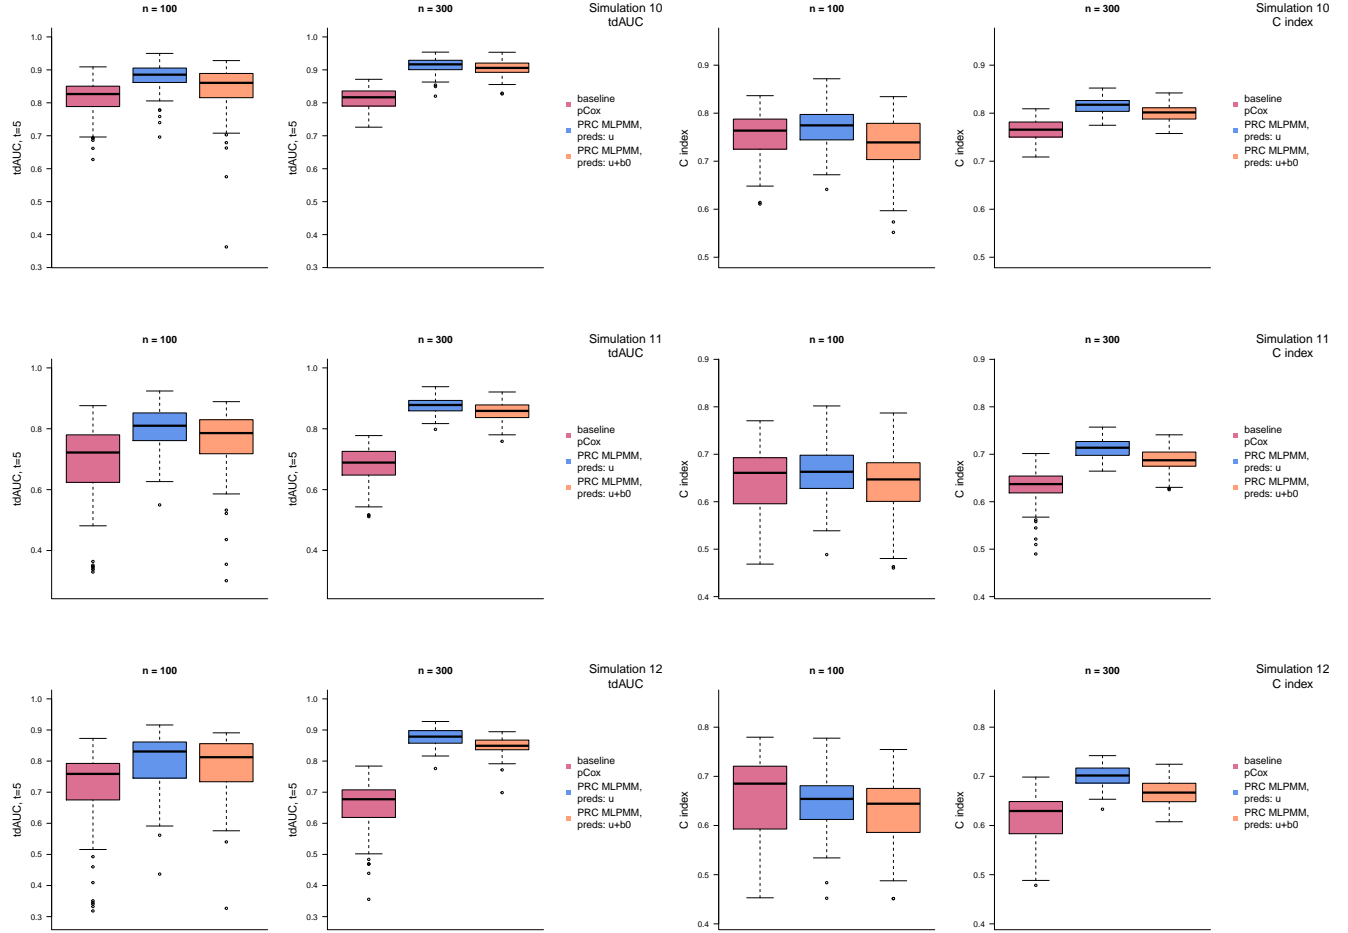

Figure 4: Results of simulations 10, 11 and 12 using the elasticnet penalty. The boxplots compare the distribution over 100 random replications of the optimism-corrected tdAUC (left) and C index (right) of the baseline pCox (violet red), PRC-MLPMM(U) (blue) and PRC-MLPMM(U+B) (orange) models.
